# Supplementary material for: Stepwise Reasoning Verification: Don't Generate, Classify!
Source: arXiv:2610.25441 source file (2026-11-01)
Supplement: Supplementary file 1 [file ARR_GUILDLINE.tex]

\section{Implementation Details}
\label{appendix:implementation}

\textit{TODO: placeholder for now...}

\section{Introduction}

These instructions are for authors submitting papers to *ACL conferences using \LaTeX. They are not self-contained. All authors must follow the general instructions for *ACL proceedings,\footnote{\url{http://acl-org.github.io/ACLPUB/formatting.html}} and this document contains additional instructions for the \LaTeX{} style files.

The templates include the \LaTeX{} source of this document (\texttt{acl\_latex.tex}),
the \LaTeX{} style file used to format it (\texttt{acl.sty}),
an ACL bibliography style (\texttt{acl\_natbib.bst}),
an example bibliography (\texttt{custom.bib}),
and the bibliography for the ACL Anthology (\texttt{anthology.bib}).

\section{Engines}

To produce a PDF file, pdf\LaTeX{} is strongly recommended (over original \LaTeX{} plus dvips+ps2pdf or dvipdf).
The style file \texttt{acl.sty} can also be used with
lua\LaTeX{} and
Xe\LaTeX{}, which are especially suitable for text in non-Latin scripts.
The file \texttt{acl\_lualatex.tex} in this repository provides
an example of how to use \texttt{acl.sty} with either
lua\LaTeX{} or
Xe\LaTeX{}.

\section{Preamble}

The first line of the file must be
\begin{quote}
\begin{verbatim}
\documentclass[11pt]{article}
\end{verbatim}
\end{quote}

To load the style file in the review version:
\begin{quote}
\begin{verbatim}
\usepackage[review]{acl}
\end{verbatim}
\end{quote}
For the final version, omit the \verb|review| option:
\begin{quote}
\begin{verbatim}
\usepackage{acl}
\end{verbatim}
\end{quote}

To use Times Roman, put the following in the preamble:
\begin{quote}
\begin{verbatim}
\usepackage{times}
\end{verbatim}
\end{quote}
(Alternatives like txfonts or newtx are also acceptable.)

Please see the \LaTeX{} source of this document for comments on other packages that may be useful.

Set the title and author using \verb|\title| and \verb|\author|. Within the author list, format multiple authors using \verb|\and| and \verb|\And| and \verb|\AND|; please see the \LaTeX{} source for examples.

By default, the box containing the title and author names is set to the minimum of 5 cm. If you need more space, include the following in the preamble:
\begin{quote}
\begin{verbatim}
\setlength\titlebox{<dim>}
\end{verbatim}
\end{quote}
where \verb|<dim>| is replaced with a length. Do not set this length smaller than 5 cm.

\section{Document Body}

\subsection{Footnotes}

Footnotes are inserted with the \verb|\footnote| command.\footnote{This is a footnote.}

\subsection{Tables and figures}

See Table~\ref{tab:accents} for an example of a table and its caption.
\textbf{Do not override the default caption sizes.}

\begin{table}
  \centering
  \begin{tabular}{lc}
    \hline
    \textbf{Command} & \textbf{Output} \\
    \hline
    \verb|{\"a}|     & {\"a}           \\
    \verb|{\^e}|     & {\^e}           \\
    \verb|{\`i}|     & {\`i}           \\
    \verb|{\.I}|     & {\.I}           \\
    \verb|{\o}|      & {\o}            \\
    \verb|{\'u}|     & {\'u}           \\
    \verb|{\aa}|     & {\aa}           \\\hline
  \end{tabular}
  \begin{tabular}{lc}
    \hline
    \textbf{Command} & \textbf{Output} \\
    \hline
    \verb|{\c c}|    & {\c c}          \\
    \verb|{\u g}|    & {\u g}          \\
    \verb|{\l}|      & {\l}            \\
    \verb|{\~n}|     & {\~n}           \\
    \verb|{\H o}|    & {\H o}          \\
    \verb|{\v r}|    & {\v r}          \\
    \verb|{\ss}|     & {\ss}           \\
    \hline
  \end{tabular}
  \caption{Example commands for accented characters, to be used in, \emph{e.g.}, Bib\TeX{} entries.}
  \label{tab:accents}
\end{table}

As much as possible, fonts in figures should conform
to the document fonts. See Figure~\ref{fig:experiments} for an example of a figure and its caption.

Using the \verb|graphicx| package graphics files can be included within figure
environment at an appropriate point within the text.
The \verb|graphicx| package supports various optional arguments to control the
appearance of the figure.
You must include it explicitly in the \LaTeX{} preamble (after the
\verb|\documentclass| declaration and before \verb|\begin{document}|) using
\verb|\usepackage{graphicx}|.

\begin{figure}[t]
  \includegraphics[width=\columnwidth]{example-image-golden}
  \caption{A figure with a caption that runs for more than one line.
    Example image is usually available through the \texttt{mwe} package
    without even mentioning it in the preamble.}
  \label{fig:experiments}
\end{figure}

\begin{figure*}[t]
  \includegraphics[width=0.48\linewidth]{example-image-a} \hfill
  \includegraphics[width=0.48\linewidth]{example-image-b}
  \caption {A minimal working example to demonstrate how to place
    two images side-by-side.}
\end{figure*}

\subsection{Hyperlinks}

Users of older versions of \LaTeX{} may encounter the following error during compilation:
\begin{quote}
\verb|\pdfendlink| ended up in different nesting level than \verb|\pdfstartlink|.
\end{quote}
This happens when pdf\LaTeX{} is used and a citation splits across a page boundary. The best way to fix this is to upgrade \LaTeX{} to 2018-12-01 or later.

\subsection{Citations}

\begin{table*}
  \centering
  \begin{tabular}{lll}
    \hline
    \textbf{Output}           & \textbf{natbib command} & \textbf{ACL only command} \\
    \hline
    \citep{Gusfield:97}       & \verb|\citep|           &                           \\
    \citealp{Gusfield:97}     & \verb|\citealp|         &                           \\
    \citet{Gusfield:97}       & \verb|\citet|           &                           \\
    \citeyearpar{Gusfield:97} & \verb|\citeyearpar|     &                           \\
    \citeposs{Gusfield:97}    &                         & \verb|\citeposs|          \\
    \hline
  \end{tabular}
  \caption{\label{citation-guide}
    Citation commands supported by the style file.
    The style is based on the natbib package and supports all natbib citation commands.
    It also supports commands defined in previous ACL style files for compatibility.
  }
\end{table*}

Table~\ref{citation-guide} shows the syntax supported by the style files.
We encourage you to use the natbib styles.
You can use the command \verb|\citet| (cite in text) to get ``author (year)'' citations, like this citation to a paper by \citet{Gusfield:97}.
You can use the command \verb|\citep| (cite in parentheses) to get ``(author, year)'' citations \citep{Gusfield:97}.
You can use the command \verb|\citealp| (alternative cite without parentheses) to get ``author, year'' citations, which is useful for using citations within parentheses (e.g. \citealp{Gusfield:97}).

A possessive citation can be made with the command \verb|\citeposs|.
This is not a standard natbib command, so it is generally not compatible
with other style files.

\subsection{References}

\nocite{Ando2005,andrew2007scalable,rasooli-tetrault-2015}

The \LaTeX{} and Bib\TeX{} style files provided roughly follow the American Psychological Association format.
If your own bib file is named \texttt{custom.bib}, then placing the following before any appendices in your \LaTeX{} file will generate the references section for you:
\begin{quote}
\begin{verbatim}
\bibliography{custom}
\end{verbatim}
\end{quote}

You can obtain the complete ACL Anthology as a Bib\TeX{} file from \url{https://aclweb.org/anthology/anthology.bib.gz}.
To include both the Anthology and your own .bib file, use the following instead of the above.
\begin{quote}
\begin{verbatim}
\bibliography{anthology,custom}
\end{verbatim}
\end{quote}

Please see Section~\ref{sec:bibtex} for information on preparing Bib\TeX{} files.

\subsection{Equations}

An example equation is shown below:
\begin{equation}
  \label{eq:example}
  A = \pi r^2
\end{equation}

Labels for equation numbers, sections, subsections, figures and tables
are all defined with the \verb|\label{label}| command and cross references
to them are made with the \verb|\ref{label}| command.

This an example cross-reference to Equation~\ref{eq:example}.

\subsection{Appendices}

Use \verb|\appendix| before any appendix section to switch the section numbering over to letters. 

\section{Bib\TeX{} Files}
\label{sec:bibtex}

Unicode cannot be used in Bib\TeX{} entries, and some ways of typing special characters can disrupt Bib\TeX's alphabetization. The recommended way of typing special characters is shown in Table~\ref{tab:accents}.

Please ensure that Bib\TeX{} records contain DOIs or URLs when possible, and for all the ACL materials that you reference.
Use the \verb|doi| field for DOIs and the \verb|url| field for URLs.
If a Bib\TeX{} entry has a URL or DOI field, the paper title in the references section will appear as a hyperlink to the paper, using the hyperref \LaTeX{} package.
