# Supplementary material for: Stepwise Reasoning Verification: Don't Generate, Classify!
Source: arXiv:2610.25441 source file (2026-11-01)
Supplement: Supplementary file 2 [file loc_acc_results.tex]

\section{First-Error Ranking Accuracy}
\label{appendix:ranking_results}

\par Step-level AUC pools scores across all instances. As a complementary check that a verifier can locate the first error within a solution, we compute ranking accuracy on trajectories that contain an annotated error: with the first error at step $k$, we predict $\hat{k}=\operatorname*{arg\,max}_{1\leq i\leq k} p_i$ and report the proportion of trajectories with $\hat{k}=k$ (Table~\ref{tab:ranking_results}).

\par The comparison between objectives is unchanged. Classification leads generation on every backbone up to 4B, by 0.021 to 0.065, and does not lead at 7B ($-0.118$ on Qwen2.5-7B and $-0.001$ on Qwen2.5-Math-7B, against $-0.073$ and $0.000$ in AUC). Qwen2.5-Math-7B is again the strongest backbone, with both objectives within 0.001 (0.882 and 0.881), and ModernBERT-B (0.805) again exceeds every generation decoder up to 4B except Qwen2.5-3B. Because the metric compares steps only within a trajectory, it can diverge from AUC for individual models: DeBERTa-B has the lowest MathShepherd AUC among encoders (0.617) but the highest ranking accuracy in that column (0.929).

\input{tabs/loc_acc_results_tab}
